# Supplementary material for: WizardMerge -- Save Us From Merging Without Any Clues
Source: arXiv:2407.02818 source file (2024-07-03)
Supplement: Supplementary file 1 [file Appendix.tex]

\section{Appendix A}

\begin{table}
\label{tb:lkdataset}
\caption{\textmd{The final datasets information for evaluations on the research questions. \textbf{Conflicts Resolved Manually} indicates the number of conflicts resolved by Git merge only. \textbf{Conflicts Analyzed By \sys} indicates the number of conflicts resolved with the assistance of \sys. \textbf{Manually Merging Time Cost} and \textbf{Merge With \sys Time Cost} show the time consumption of merging these conflicts and the violated DCBs related to these conflicts w/ or w/o \sys respectively (accurate to minutes). }}

\begin{threeparttable}
\begin{tabular}{lllll}
\toprule
Dataset ID & MCR & ACR          & MCR TC & ACR TC          \\ \midrule
LK1        & 1                           & 1                                   & 10                         & 5                                  \\
LK2        & 2                           & 2                                   & 31                         & 18                                 \\
LK3        & 5                           & 5                                   & 8                          & 5                                  \\
LK4        & 2                           & 2                                   & 5                          & 4                                  \\
LK5        & 5                           & 3                                   & 15                         & 10                                 \\
LK6        & 1                           & 1                                   & 3                          & 2                                  \\
LK7        & 2                           & 2                                   & 4                          & 4                                  \\
LK8        & 1                           & 1                                   & 2                          & 2                                  \\
LK9        & 1                           & 1                                   & 4                          & 4                                  \\
LK10       & 1                           & 1                                   & 2                          & 2                                  \\
LK11       & 4                           & 4                                   & 40                         & 33                                 \\
LK12       & 2                           & 2                                   & 6                          & 7                                  \\
LK13       & 1                           & 1                                   & 15                         & 8                                  \\
LK14       & 1                           & 1                                   & 8                          & 10                                 \\
LK15       & 1                           & 1                                   & 3                          & 3                                  \\
LK16       & 1                           & 1                                   & 1                          & 1                                  \\
LK17       & 1                           & 1                                   & 12                         & 11                                 \\
LK18       & 2                           & 2                                   & 2                          & 2                                  \\
LK19       & 2                           & 2                                   & 5                          & 10                                 \\
LK20       & 1                           & 1                                   & 1                          & 1                                  \\
LK21       & 1                           & 1                                   & 1                          & 1                                  \\
LK22       & 1                           & 1                                   & 1                          & 1                                  \\
LK23       & 2                           & 1                                   & 3                          & 2                                  \\
LK24       & 9                           & 6                                   & 30                         & 19                                 \\
LK25       & 5                           & 4                                   & 18                         & 13                                 \\
LK26       & 2                           & 2                                   & 3                          & 2                                  \\
LK27       & 1                           & 1                                   & 3                          & 3                                  \\
LK28       & 2                           & 2                                   & 2                          & 1                                  \\
LK29       & 1                           & 1                                   & 4                          & 3                                  \\
LK30       & 2                           & 2                                   & 8                          & 3                                  \\
LK31       & 1                           & 1                                   & 6                          & 4                                  \\
LK32       & 1                           & 1                                   & 1                          & 1                                  \\
LK33       & 1                           & 1                                   & 1                          & 1                                  \\
LK34       & 4                           & 4                                   & 10                         & 6                                  \\
LK35       & 1                           & 1                                   & 1                          & 1                                  \\
LK36       & 1                           & 1                                   & 2                          & 2                                  \\
LK37       & 1                           & 1                                   & 4                          & 4                                  \\
LK38       & 1                           & 1                                   & 1                          & 1                                  \\
LK39       & 1                           & 1                                   & 1                          & 1                                  \\
LK40       & 7                           & 7                                   & 10                         & 6                                  \\
LK41       & 1                           & 0                                   & 1                          & /                                  \\
LK42       & 2                           & 0                                   & 3                          & /                                  \\
LK43       & 3                           & 0                                   & 2                          & /                                  \\  \bottomrule
\end{tabular}

\begin{tablenotes}
\footnotesize
\item[1] \sys-Async-CG1: \sys ablation control group one. The statistics are recorded with \sys running without multi-threaded constraint solving.
% \item[2] \sys-Async-CG2: \sys ablation control group two. The statistics are recorded with \sys running without state sharing between fuzzer and concolic executor backend.
\end{tablenotes}
\end{threeparttable}

\end{table}
\begin{table}
\label{tb:ffdataset}
\caption{\textmd{The final datasets information for evaluations on the research questions. \textbf{Conflicts Resolved Manually} indicates the number of conflicts resolved by Git merge only. \textbf{Conflicts Analyzed By \sys} indicates the number of conflicts resolved with the assistance of \sys. \textbf{Manually Merging Time Cost} and \textbf{Merge With \sys Time Cost} show the time consumption of merging these conflicts and the violated DCBs related to these conflicts w/ or w/o \sys respectively (accurate to minutes). }}

\begin{threeparttable}
\begin{tabular}{lllll}
\toprule
Dataset ID & MCR & ACR          & MCR TC & ACR TC          \\ \midrule
FF1        & 2                           & 2                                   & 3                          & 2                                  \\
FF2        & 2                           & 1                                   & 11                         & 6                                  \\
FF3        & 12                          & 12                                  & 49                         & 28                                 \\
FF4        & 11                          & 11                                  & 8                          & 5                                  \\
FF5        & 25                          & 25                                  & 32                         & 22                                 \\
FF6        & 26                          & 26                                  & 30                         & 27                                 \\
FF7        & 13                          & 13                                  & 42                         & 25                                 \\
FF8        & 3                           & 3                                   & 13                         & 8                                  \\
FF9        & 2                           & 2                                   & 2                          & 2                                  \\
FF10       & 9                           & 9                                   & 10                         & 10                                 \\
FF11       & 2                           & 2                                   & 4                          & 4                                  \\
FF12       & 3                           & 3                                   & 4                          & 3                                  \\
FF13       & 8                           & 8                                   & 16                         & 12                                 \\
FF14       & 1                           & 1                                   & 1                          & 1                                  \\
FF15       & 2                           & 2                                   & 2                          & 2                                  \\
FF16       & 1                           & 1                                   & 1                          & 1                                  \\
FF17       & 6                           & 6                                   & 6                          & 5                                  \\
FF18       & 12                          & 12                                  & 30                         & 19                                 \\
FF19       & 1                           & 1                                   & 1                          & 1                                  \\
FF20       & 3                           & 3                                   & 13                         & 8                                  \\
FF21       & 13                          & 13                                  & 59                         & 43                                 \\
FF22       & 3                           & 3                                   & 5                          & 4                                  \\ \bottomrule
\end{tabular}

\begin{tablenotes}
\footnotesize
\item[1] \sys-Async-CG1: \sys ablation control group one. The statistics are recorded with \sys running without multi-threaded constraint solving.
% \item[2] \sys-Async-CG2: \sys ablation control group two. The statistics are recorded with \sys running without state sharing between fuzzer and concolic executor backend.
\end{tablenotes}
\end{threeparttable}

\end{table}
